# Supplementary material for: ShareCMP: Polarization-Aware RGB-P Semantic Segmentation
Source: arXiv:2312.03430 source file (2025-07-04)
Supplement: Supplementary file 1 [file appendix.tex]

\clearpage
\setcounter{page}{1}
\maketitlesupplementary

% \href{address}{text}
